# Supplementary material for: GNNBENCH: Fair and Productive Benchmarking for Single-GPU GNN System
Source: arXiv:2404.04118 source file (2024-04-05)
Supplement: Supplementary file 1 [file SM.tex]

\subsection{{\myname-SM}: Graph Preparation and Exchange} \label{sec.engg}

The independent nature of {\myname-System} allows it to offer native Python binding capabilities. Hence, by modeling a graph as a class object, any custom graph storage can now be passed to its APIs using the same object, hence achieving a stable API. It is much better than using tensors to model graphs that needed workarounds and unstable APIs. 

Apart from customizing the graph storage format, one more variation in graph storage can be observed based on the edge properties.
%\noindent \textbf{Challenges.}
%\noindent \textbf{Gap between C/C++ and Python.}
To illustrate, edges are unweighted and undirected in GCN and GIN  but contain edge ID and are directed in the case of GAT.
%as each edge stores a trainable weight whose access is required through edge ID indirection.
%GAT requires introducing the edge ID abstraction for each edge where the edge ID points the offset in an attention score array to read (forward computation) and modify (backward computation that uses reverse graph) the attention score. 
Furthermore, graph edge requires an edge type being stored as well apart from the edge ID for the knowledge graph auto-completion GNNs~\cite{rgcn2018}. 
%Similarly, sparse tensors require the support of bipartite graphs and edge ID.
Not to mention, the ad hoc data science use-case may require the support of arbitrary multi-field properties, e.g., In LANL network dataset~\cite{turcotte17}, each edge has 9 fields and requires 32 bytes. 
%Similarly, a vertex can have properties, including its string-based identifier, type in the heterogeneous graph, timestamp, etc.

The research question here is whether we can pass graph storage with diverse edge properties to {\myname-System} for various use cases using stable APIs.
Moreover, the next opportunity to develop a productive GNN framework is to allow passing prepared graph to {\myname-System} directly and not forcing it to do the mundane tasks of file handling, data parsing, and parallel processing. 
Hence, another independent module handling graph creation is desired, and it can also be used for other graph data science use cases.

\subsubsection{Edge Property Specification: Numpy Dtype}
%\noindent \textbf

{\myname} relies on \textit{Numpy dtype} for edge property specification in the interfaces. 
%and each additional edge property can easily be modeled by defining the dtype. 
Hence, like a NumPy array object, a graph object can also allow the passing of diverse edge properties as shown in Listing~\ref{list-dtype}.
The Numpy dtype is a data type object which looks like a C-structure in Python but keeps many other details like the size of the array elements. Each element can be a native type, such as \textit{float} for a Numpy array of single floating points, or it can be a multi-field (e.g. edge weight, edge ID, edge type, etc.), each with a fixed size data type. 
%allow data scientists to define any arbitrary edge properties in Python, while {\graphpy-SM} dynamically supports those properties without any changes or compilation.
It should be noted that the dtype mechanism has become a de-facto standard for tensor specification in Python, though DL frameworks only allow a few dtype. \textit{{\myname} offers the exchange of graph objects among different modules by using the same de-facto standard of dtype resulting in stable APIs.}

%The {\graphpy-GNN} then can do any additional pre-processing to generate a custom graph storage. 
%Therefore how the interfaces should be designed to allow passing such diverse graphs to {\graphpy-GNNs} so that each can keep its own custom storage with the single notion of graph object to unify the model layer definition and training without redefining everything from scratch for changes to graph storage or format? 

Numpy dtype can specify many properties, and hence C++ ideally needs a new \textit{class} definition to support their compilation. 
%Differences between Python (interpreter-based language) and C++ (compiler-based language) environments introduce an important challenge to support graphs with arbitrary properties. 
For example, we can use 
%GraphOne~\cite{kumar2017graphone}, which uses 
template meta-programming to define edge properties using a C++ \textit{struct}, and can write a Python binding for the same. However, each custom property requires a new  definition in C++, and new Python binding, followed by \textit{compiling} it for use in Python.
% However, we realize that the job of {\graphpy-SM} is just to prepare the graph and not to provide graph analysis, which may require the definition of real classes to access property fields in a C++ way. 
However, dtype is nothing but information about how an array element should be interpreted in Python, including the size and type of each element in the array. 
%Hence, it is very easy to go to a specific element to read or write to it, if back-end can store the dtype information, including the size of each field. 
% Also, it is very easy to parse the input files and perform the tokenization to support reading a good set of raw input files and preparing the graph representation from it.
Hence, {\myname-SM} uses void pointers, element size, and other information to support dtype, along with a convention that edge dtype should always specify the source vertex first, destination vertex next, then the edge properties. Hence, by knowing the size of the edge properties, we can easily prepare a graph in {\myname-SM} without defining the actual C++ structure for the same.

\subsubsection{Graph Preparation, Exchange, and Ownership.} 
Table~\ref{table-api} lists graph storage related APIs. Listing ~\ref{list-dtype} shows an example of how {\myname-SM} prepares graph representation from the user-defined edge structure using Python dtype, and passes the prepared graph to {\myname-System}. The {\myname-SM} uses multiple cores and can generate the optional edge ID. The parsing APIs \textit{$add\_edges\_from\_*$()} accept delimiters and flags to support different types of input files.
For complex input data format, we require that users directly parse using the Python IO library, and send the back-end a Numpy array of edges in batches or at once using \textit{add$\_$edges()} API. Python has very good APIs for file handling and tokenization.

\begin{table}[t]
\caption{\small {\myname} Python APIs for Graph Storage Handling} % title of Table
\vspace{-6pt}
\centering \small % used for centering table
\begin{tabular}{|l| l l } % centered columns (4 columns)
    \hline %inserts a single line
     \textbf{{\myname-SM} Initialization APIs} \\
    \hline
%    graph \hspace{1mm} init() \\
%   \hline
 %   $vclass$  init$\_$vclass(vertex$\_$count, vclass$\_$name, flag)\\
%   \hline
    $G$ \hspace{2mm} init$\_$graph(vcount, flag, edge$\_$dtype, graph$\_$name) \\
%    \hspace{22mm} e$\_$dtype, graph$\_$name)\\
    \hline
    \textbf{Graph Preparation APIs of {\myname-SM} on $G$} \\
    \hline %inserts double horizontal lines
    int \hspace{1mm} add$\_$edges$\_$from$\_$file(file$\_$name, delimiter, flag)\\
    int \hspace{1mm} add$\_$edges$\_$from$\_$dir(dir$\_$name, delimiter, flag) \\
    int \hspace{1mm} add$\_$edges(np$\_$array, count) \Comment{\blue{Can be called many times}}\\
    \hline %inserts a single line
    \textbf{Some APIs of {\myname-SM} on $G$}\\
    \hline
    {np$\_$arr1, np$\_$arr2, np$\_$arr3, np$\_$arr4} \hspace{1mm} get$\_$csr(csr$\_$dtype) \\
    %\hline
    %{Numpy$\_$array, Numpy$\_$array} \hspace{1mm} get$\_$csc(graph, dtype) \\
    %\hline
%    np$\_$array \hspace{16mm} get$\_$coo(edge$\_$dtype)\\
    \hline
    % \hspace{6mm} \textbf{ Vertex Related APIs of $vclass$} \\
    % \hline
    % int \hspace{5mm} string$\_$to$\_$vid(vertex$\_$name) \\
    % string \hspace{1mm} vid$\_$to$\_$string(vid) \\
    % \hline
    \textbf{Some Graph APIs of {\myname-System}} \\
    \hline
    g  \hspace{12mm} wrap$\_$graph(np$\_$arr1, np$\_$arr2, np$\_$arr3, np$\_$arr4) \\
    status \hspace{6mm} save$\_$graph(g, path) \\
    g \hspace{12mm} load$\_$graph(path) \\
    vcount \hspace{5mm} get$\_$vcount() \\
    ecount \hspace{5mm} get$\_$ecount() \\
     \hline
\end{tabular}
\label{table-api} % is used to refer this table in the text
% \vspace{-12pt}
\end{table}

\begin{lstlisting}[language=Python, caption= {\small Illustration of graph creation in Python using {\myname-SM} and passing it to a {\myname-System}. Edges have one property.}, label={list-dtype}]
import Numpy as np
import gnnbench_sm as gp
import gnnbench_kernel as gpk
def prep_graph():
 edge_dt=np.dtype([('src', np.int32), ('dst', np.int32), ('eid', np.int32)]
 csr_dt=np.dtype([('dst', np.int32), ('eid', np.int32)]) #dtype for csr
 G = gp.init_graph(|V|,edge_dt,"reddit", gp.eDir)
 G.add_edges_from_dir('./InputDir/', ' ', gp.eEid)
 g = gpk.wrap_graph(G.get_csr(csr_dt))
\end{lstlisting}

%\vspace{-6pt}

% V = init_vclass(vcount, "vclass1", 0)
%csr_offset, csr_neighbor, csc_offset, csc_neighbor 
%kernel_graph = gpk.wrap_graph(csr_offset, csr_neighbor, csc_offset, csc_neighbor);

{\myname-SM} exports the graph in CSR/CSC in the form of four zero-copy NumPy arrays using \textit{get$\_$csr()} API (At Line 9). The first Numpy array contains the \textit{offset} of size $|V+1|$, while the second array contains N(v) of the vertices along with the embedded edge properties as specified using dtype. The rest of the two arrays are for CSC format. In the case of an undirected graph, both groups of NumPy arrays share the same underlying memory. The four arrays are sufficient to pass any CSC/CSR variants taking care of the direction, edge IDs, or any multi-field property, etc. 

These arrays can be passed to the $wrap\_graph$() API of the \myname-GNN (Line 9) to initialize its internal graph wrapping these arrays or may further pre-process the graph to derive a new format and return the kernel-graph object(g) which is used by other {\myname-System} APIs. 
%The {\graphpy-GNN} can simply store the underlying memory pointers as offset and neighbor arrays inside the  kernel-graph object to offer vanilla CSR/CSC; or may decide to further pre-process the graph to derive a new format, and return the corresponding kernel-graph object. 
%based on parameters being passed through $dict\_param$, a python dictionary data-type, 
Thus, the kernel-graph object is owned by {\myname-System}. The module can save it to disk ($save\_graph()$ API in Table~\ref{table-api}), or load it from there ($load\_graph()$ API in Table~\ref{table-api}) without affecting {\myname-SM} or its other consumers (\cref{sec.overview}). 
