# Supplementary material for: GNNBENCH: Fair and Productive Benchmarking for Single-GPU GNN System
Source: arXiv:2404.04118 source file (2024-04-05)
Supplement: Supplementary file 2 [file appendix.tex]

\newpage

\appendix

\subsection{Versatility of {\myname}}

%\textbf{Easily applicable to multiple DL framework}
{\myname} can integrate with multiple DL frameworks, such as Pytorch, Tensorflow, and MXNet easily. While the majority of our experimental results are evaluated using the PyTorch integration, we also demonstrate compatibility with TensorFlow for GCN to show that integration with any general-purpose DL framework is possible that offers DLPacktensors. Table.\ref{table-graphpy-TFvsPT} shows that Pytorch and Tensorflow integration achieve similar accuracy.

\begin{table}[h]
\small
\vspace{-6pt}
\caption{\small {\myname}-TensorFlow vs {\myname}-PyTorch accuracy comparison for GCN by integrating Cusparse.} % title of Table
\vspace{-6pt}
\centering % used for centering table
\begin{tabular}{|l| r| r|} % centered columns (4 columns)
    \hline\hline %inserts double horizontal lines
    Graph Dataset & {\myname}-Tensorflow & {\myname}-Pytorch\\ [0.5ex] % inserts table
    %heading
    \hline % inserts single horizontal line
    Cora & 83.18\% &  83.40\%\\ 
    Citeseer & 65.32\% & 65.10\%  \\
    PubMed & 76.47\% &  76.52\%\\
    Reddit & 92.89\% &  92.96\%\\
    OGB-Product & 69.76\%& 69.67\%\\
    % Kron-20 & 1,048,576 & 10,485,760\\
    % [1ex] % [1ex] adds vertical space
    \hline %inserts single line
\end{tabular}
\vspace{-6pt}
\label{table-graphpy-TFvsPT} % is used to refer this table in the text
\end{table}

\subsection{Other supporting materials}

 This section presents our code-study results to show that many prior works have pitfalls. These are supporting materials and are optional to convince that pitfalls exist, requiring benchmarking systems. Camera-ready version will not have these materials, as they are part of another paper that has formalized the pitfalls and is under review at another conference. Kindly note that we have reached to authors of their papers to get a confirmation. They all have agreed on the issue, though some have also emphasized that the DGL and Cusparse codebase have evolved.

\subsubsection{GNNAdvisor} \url{https://github.com/YukeWang96/GNNAdvisor_OSDI21/blob/master/GNNAdvisor/GNNConv/GNNAdvisor_kernel.cu#L542} points to backward propagation which performs the SpMMv first, then the normalization part within the same kernel. The forward also performs these operations in the same order(line 403), and hence backward should have been done in reverse order. 

\url{https://github.com/YukeWang96/GNNAdvisor_OSDI21/blob/master/GNNAdvisor/gnn_conv.py#L98} shows that the bias operator is not there. \url{https://github.com/dmlc/dgl/blob/master/python/dgl/nn/pytorch/conv/graphconv.py#L206} shows that the bias operator is set as True by default in DGL. But \url{https://github.com/YukeWang96/GNNAdvisor_OSDI21/blob/master/dgl_baseline/gcn.py#L12} shows GNNAdvisor did not specifically disable bias in DGL. 

\subsubsection{TC-GNN} 

\url{https://github.com/YukeWang96/TC-GNN_ATC23/blob/atc23ae/TCGNN_conv/TCGNN_kernel.cu#L336} and \url{https://github.com/YukeWang96/TC-GNN_ATC23/blob/atc23ae/gnn_conv.py} shows that TC-GNN's GCN implementation does not include normalization by degree and bias operator either in the kernel or in Python. But these two URLs (\url{https://github.com/YukeWang96/TC-GNN_ATC23/blob/atc23ae/dgl_baseline/gcn.py#L20} \url{https://github.com/dmlc/dgl/blob/master/python/dgl/nn/pytorch/conv/graphconv.py#L197}) show that TC-GNN uses the default setting for bias and normalization in DGL. This means their DGL baseline enables both the normalization and bias operator. 

One can also see that its AGNN (\url{https://github.com/YukeWang96/TC-GNN_ATC23/blob/atc23ae/TCGNN_conv/TCGNN_kernel.cu} ) kernels don't do tranpose at all during backward pass. 

\subsubsection{FuseGNN} 

\url{https://github.com/apuaaChen/gcnLib/issues/3} reported an accuracy issue in Github but got no response. Our measurements also show the same accuracy issue. 

\subsubsection{Huang et al} 

\url{https://github.com/xxcclong/GNN-Computing/blob/master/include/aggr_gat.h}  There is no transpose SpMM function implemented, the kernels work fine for forward but are not workable for backward pass. Their Python code also does not explicitly call/have transposed API from Pytorch/Cusparse. 

It uses the same copy of edge-level tensor for all the layers of GAT. Hence, in the real-world, they would not be usable in backward propagation. The correct approach would have been to allocate separate memory for each edge-level tensor.  

The kernel does not work when the dim is not a multiple of 32, which is a common case for the last layer of GAT. E.g., in Reddit and ogb-product, the feature dimensions are 41 and 47 respectively. 

For GCN: \url{https://github.com/xxcclong/GNN-Computing/blob/master/include/aggr_gcn.h} shows that all the kernels here require an edge-level tensor, i.e. this paper provides SpMMve and not SpMMv, and is the main reason for slower performance despite having a workload-balanced solution. 

The kernel does not work for odd dimensions, which is a common occurrence for GCN, specifically for the last layer. E.g., 6 for Cora. 

\subsubsection{TLPGNN} 

\url{https://github.com/charlifu/TLPGNN/blob/main/gat/kernel.cu#L49} shows the fused kernel for GAT forward where the attention-score (edge-level tensor) is computed and stored in a register and not materialized in GPU global memory. 

It also neither has backward code for GAT nor transpose code anywhere. 

\subsubsection{Seastar} 

Seastar does not have its code in Github, but it provides a URL to download it. Upon running its training script, it generates the kernel code (in CUDA), compiles it (all automatically), and runs training. We read the generated GCN sparse kernel, which generates a fused version of SpMMv and normalization by degree, and suffered from the same set of issues as discussed for GNNAdvisor. 

\subsubsection{DGL} 

We have reached out to DGL recently through a long email. We are yet to hear from the person. Before this, we had a face-to-face meeting with this person in a conference/workshop, and the employee indicated that they acknowledge that DGL suffers from some issues that we highlighted in the paper. At that time, the manuscript was not fully ready.
